# Supplementary material for: Improving Cross-Lingual Token Representations by Adding a Pinch of SALT
Source: arXiv:2609.09953 source file (2026-11-18)
Supplement: Supplementary file 2 [file 999_appendix_old.tex]

\section{Case algorithm}
\begin{algorithm}
\caption{CASE span extraction}
\label{case}
\begin{algorithmic}[1]
\State $\textit{maps} \gets \text{Argmax}(x, y, \mathcal{E})$
\State $\textit{constituents} \gets \text{ConstituentTagger}(x)$
\State $\textit{valid\_spans} \gets \emptyset$
\For{each $\textit{source\_span}$ in $\textit{constituents}$}
    \State $\textit{tgt\_indices} \gets \emptyset$
    \For{each token $t$ in $\textit{source\_span}$}
        \If{$t \in \textit{maps}$}
            \State append $\textit{maps}[t]$ to $\textit{tgt\_indices}$
        \EndIf
    \EndFor
    \If{$\textit{tgt\_indices} = \emptyset$}
        \State \textbf{continue} \Comment{no mapped tokens, discard span}
    \EndIf
    \State $\textit{target\_span} \gets [\min(\textit{tgt\_indices}),\, \max(\textit{tgt\_indices})]$
    \For{each token $s$ in $\textit{target\_span}$}
        \If{mapping of $s$ in $x$ is outside $\textit{source\_span}$}
            \State \textbf{continue} to next $\textit{source\_span}$ \Comment{discard span}
        \EndIf
    \EndFor
    \State $\textit{src\_mapped} \gets$ \# tokens in $\textit{source\_span}$ with mappings in $y$
    \State $\textit{tgt\_mapped} \gets$ \# tokens in $\textit{target\_span}$ with mappings in $x$
    \State $\textit{coverage} \gets (\textit{src\_mapped} + \textit{tgt\_mapped})\;/\;(|\textit{source\_span}| + |\textit{target\_span}|)$
    \If{$\textit{coverage} > c$}
        \State add $(\textit{source\_span},\, \textit{target\_span})$ to $\textit{valid\_spans}$
    \EndIf
\EndFor
\State \Return $\textit{valid\_spans}$
\end{algorithmic}
\end{algorithm}
